# Supplementary material for: Attribute Exploration with Multiple Contradicting Partial Experts
Source: arXiv:2205.15714 source file (2022-05-31)
Supplement: Supplementary file 1 [file explorationtables.tex]

\begin{table}
\centering
\begin{tabular}{|lc| cccc |l|}
\hline
Implication & m & APP.1.1 & CON.1 & ORP.1 & SYS.1.1 & Counterexamples \\
\hline
$\emptyset$ $\rightarrow$ (18 19 20 21 22) & &&&& & \\
 &  18  & .  & .  & .  & . & A16, C11, O04, S06 \\
 &  19  & .  & .  & x  & . & A16, C14, S01 \\
 &  20  & .  & .  & .  & . & A02, C03, O13, S06 \\
 &  21  & .  & .  & .  & . & A16, C11, O13, S35 \\
 &  22  & .  & .  & .  & . & A06, C11, O16, S35 \\
(21) $\rightarrow$ (18 20) & &&&& & \\
 &  18  & .  & .  & x  & . & A11, C16, S21 \\
 &  20  & x  & .  & x  & . & C16, S21 \\
(20 21 22) $\rightarrow$ (18 19) & &&&& & \\
 &  18  & x  & x  & x  & . & S31 \\
 &  19  & x  & x  & x  & . & S31 \\
(19 21) $\rightarrow$ (18 20 22) & &&&& & \\
 &  18  & x  & x  & x  & . & S34 \\
 &  20  & x  & x  & x  & . & S34 \\
 &  22  & x  & x  & x  & x &  \\
(19 20 22) $\rightarrow$ (18 21) & &&&& & \\
 &  18  & .  & x  & x  & x & A15 \\
 &  21  & .  & x  & x  & x & A15 \\
(19 20 21 22) $\rightarrow$ (18) & &&&& & \\
 &  18  & x  & x  & x  & x &  \\
(18 22) $\rightarrow$ (19) & &&&& & \\
 &  19  & x  & x  & x  & x &  \\
(18 21) $\rightarrow$ (20) & &&&& & \\
 &  20  & x  & x  & x  & x &  \\
(18 19 20 22) $\rightarrow$ (21) & &&&& & \\
 &  21  & x  & x  & x  & x &  \\
\hline
\end{tabular}
\caption{ Exploration of the shared implications of  APP.1.1, CON.1, ORP.1, SYS.1.1 }
\label{ appendix-exploration- APP.1.1-CON.1-ORP.1-SYS.1.1 }
\end{table}

\begin{table}
\centering
\begin{tabular}{|lc| ccc |l|}
\hline
Implication & m & CON.1 & ORP.1 & SYS.1.1 & Counterexamples \\
\hline
(20 22) $\rightarrow$ (21) & &&& & \\
 &  21   & x  & x  & x &  \\
(20 21) $\rightarrow$ (22) & &&& & \\
 &  22   & x  & x  & x &  \\
(18) $\rightarrow$ (19) & &&& & \\
 &  19   & .  & x  & . & C15, S13 \\
(18 20) $\rightarrow$ (19) & &&& & \\
 &  19   & .  & x  & . & C09, S11 \\
\hline
\end{tabular}
\caption{ Exploration of the shared implications of  CON.1, ORP.1, SYS.1.1 }
\label{ appendix-exploration- CON.1-ORP.1-SYS.1.1 }
\end{table}

\begin{table}
\centering
\begin{tabular}{|lc| ccc |l|}
\hline
Implication & m & APP.1.1 & CON.1 & SYS.1.1 & Counterexamples \\
\hline
(18 19) $\rightarrow$ (20) & &&& & \\
 &  20  & .  & .   & x & A12, C07 \\
(18 19 22) $\rightarrow$ (20 21) & &&& & \\
 &  20  & x  & x   & x &  \\
 &  21  & x  & x   & x &  \\
\hline
\end{tabular}
\caption{ Exploration of the shared implications of  APP.1.1, CON.1, SYS.1.1 }
\label{ appendix-exploration- APP.1.1-CON.1-SYS.1.1 }
\end{table}

\begin{table}
\centering
\begin{tabular}{|lc| ccc |l|}
\hline
Implication & m & APP.1.1 & CON.1 & ORP.1 & Counterexamples \\
\hline
(18 19 20) $\rightarrow$ (21 22) & &&& & \\
 &  21  & x  & .  & x  & C04 \\
 &  22  & x  & .  & x  & C04 \\
\hline
\end{tabular}
\caption{ Exploration of the shared implications of  APP.1.1, CON.1, ORP.1 }
\label{ appendix-exploration- APP.1.1-CON.1-ORP.1 }
\end{table}

\begin{table}
\centering
\begin{tabular}{|lc| cc |l|}
\hline
Implication & m & ORP.1 & SYS.1.1 & Counterexamples \\
\hline
(19 20) $\rightarrow$ (18) & && & \\
 &  18    & x  & x &  \\
\hline
\end{tabular}
\caption{ Exploration of the shared implications of  ORP.1, SYS.1.1 }
\label{ appendix-exploration- ORP.1-SYS.1.1 }
\end{table}

\begin{table}
\centering
\begin{tabular}{|lc| cc |l|}
\hline
Implication & m & CON.1 & ORP.1 & Counterexamples \\
\hline
(21) $\rightarrow$ (22) & && & \\
 &  22   & x  & x  &  \\
\hline
\end{tabular}
\caption{ Exploration of the shared implications of  CON.1, ORP.1 }
\label{ appendix-exploration- CON.1-ORP.1 }
\end{table}

\begin{table}
\centering
\begin{tabular}{|lc| cc |l|}
\hline
Implication & m & APP.1.1 & ORP.1 & Counterexamples \\
\hline
(19 20) $\rightarrow$ (22) & && & \\
 &  22  & .   & x  & A17 \\
(18 20) $\rightarrow$ (21) & && & \\
 &  21  & x   & x  &  \\
\hline
\end{tabular}
\caption{ Exploration of the shared implications of  APP.1.1, ORP.1 }
\label{ appendix-exploration- APP.1.1-ORP.1 }
\end{table}

\begin{table}
\centering
\begin{tabular}{|lc| c |l|}
\hline
Implication & m & SYS.1.1 & Counterexamples \\
\hline
(22) $\rightarrow$ (21) & & & \\
 &  21     & . & S02 \\
\hline
\end{tabular}
\caption{ Exploration of the shared implications of  SYS.1.1 }
\label{ appendix-exploration- SYS.1.1 }
\end{table}

\begin{table}
\centering
\begin{tabular}{|lc| c |l|}
\hline
Implication & m & ORP.1 & Counterexamples \\
\hline
$\emptyset$ $\rightarrow$ (19) & & & \\
 &  19    & x  &  \\
\hline
\end{tabular}
\caption{ Exploration of the shared implications of  ORP.1 }
\label{ appendix-exploration- ORP.1 }
\end{table}
